# Supplementary material for: SceneGraphLoc: Cross-Modal Coarse Visual Localization on 3D Scene Graphs
Source: arXiv:2404.00469 source file (2024-07-12)
Supplement: Supplementary file 1 [file supplementary.tex]

\documentclass[runningheads]{llncs_supp}
\usepackage[review,year=2024,ID=1255]{eccv_supp}
% Other packages
% Commonly used abbreviations (\eg, \ie, \etc, \cf, \etal, etc.)
\usepackage{eccvabbrv}
\usepackage{graphicx}
\usepackage{booktabs}
\usepackage[accsupp]{axessibility}
% Hyperref package
\usepackage[pagebackref,breaklinks,colorlinks]{hyperref}
\usepackage{orcidlink}
\usepackage{multirow}
\usepackage{amsmath}
\usepackage{amssymb}
\usepackage{amsfonts} 
\usepackage{textcomp}
\usepackage{arydshln}
\usepackage{stmaryrd}
\usepackage{mathrsfs}
\input{macros}

\begin{document}
\title{Supplementary Material \\
SceneGraphLoc}
\author{}
\date{}
\maketitle
% reset the number for the supp. tables , equations and so on
\setcounter{table}{4}
\setcounter{table}{4}
\setcounter{figure}{5}
\setcounter{equation}{8}
\input{sections_supp/00_abstraction}
\input{sections_supp/01_qualitative_results}
\input{sections_supp/02_albation_study}
\input{sections_supp/03_impl_details}

% ---- Bibliography ----
%
% BibTeX users should specify bibliography style 'splncs04'.
% References will then be sorted and formatted in the correct style.
%
\clearpage
\bibliographystyle{splncs04}
\bibliography{egbib}

\end{document}
